# Supplementary material for: Differentially private sliced inverse regression in the federated paradigm
Source: arXiv:2306.06324 source file (2023-08-10)
Supplement: Supplementary file 1 [file Appendix-1.tex]

\subsection*{General}

\begin{lemma}\label{lem1}
Suppose that $(x, y)$ are defined over $\sigma$-finite space $\mathcal{X} \times \mathcal{Y}$ and $x$ is sub-Gaussian with mean 0 and upper exponentially bounded by $\tau$, let ${m}(y) = {E}(x|y)$, $\epsilon(y) = x - {m}(y)$, then we have 

$i)$ ${m}(y)$ and $\epsilon(y)$ are sub-Gaussian and upper-exponentially bounded by $\tau$ and $2\tau$ respectively.

$ii)$ For any fixed positive constants $C_1 < 1 < C_2$ and any partition $\mathbb{R} = \cup_{h=1}^{H}S_h$ where $S_h$ are intervals satisfying 
\begin{align*}
\frac{C_1}{H} \leq \pr(y \in S_h) \leq \frac{C_2}{H}, \forall h,
\end{align*}
there exists a constant $C$ such that 
\begin{align*}
\sup_{h}\pr(x|_{y \in S_h} > t) \leq CH \exp(1 - \frac{t^2}{\tau^2}).
\end{align*}
As a direct corollary, we know that there exists a positive constant $C$ such that
\begin{align*}
{E}\left[\exp \left\{\frac{\left(x|_{y \in S_{h}}\right)^{2}}{2 \tau^{2}}\right\}\right] \leq C H,
\end{align*}
and
\begin{align*}
{E}\left\{\left|\left(x|_{y \in S_{h}}\right)\right|^{m}\right\} \leq C H m \tau^{m} \Gamma(\frac{m}{2}) / 2.
\end{align*}

$iii)$ Suppose that $x|_{y \in S_h}$ is defined as in $ii)$. Let $x_i$, $i = 1,\dots, n_0$ be $n_0$ samples from $x|_{y \in S_h}$, $\bar{x}_{h} = (1/n_0)\sum_i^{n_0} x_i$ and $\mu_h = {E}(x|_{y \in S_h})$, we have 
\begin{align*}
P\left(\left|\bar{x}_{h}-\mu_{h}\right|>t\right) \leq 2 \exp \left(\frac{-n_0 t^{2}}{2 C H \tau ^{2}+2 t \tau}\right).
\end{align*}
\end{lemma}

\begin{proof}[of Lemma~\ref{lem1}]
This Lemma is from Lemma 17 of \cite{lin2018consistency}, thus we omit the proof here.
\end{proof}

\begin{lemma}\label{lem2}
Let $x \in \mathbb{R}^p$ be a sub-Gaussian random variable which is upper exponentially bounded by $\tau$.  For any unit vector $\beta \in \mathbb{R}^p$, let $x(\beta) = \langle x, \beta \rangle$ and ${m}(\beta) = \langle {m}, \beta \rangle = {E}\{x(\beta)|y\}$, and let $\mu_h = {E}(x|_{y \in S_h})$, then there exist a $h \in [H]$ and $\nu > 1$ such that 
\begin{align*}
|\mu_h(\beta)| \geq C_{\mu} s^{-\frac{\omega}{2}}
\end{align*}
occurs with probability at least
\begin{align*}
1 - C_1 \exp\{-C_2 \frac{n_0 s^{-\omega}}{H\nu^2} + C_3 \log{(H)}\},
\end{align*}
where $n_0$ is the sample size of the $h$th slice.
\end{lemma}

\begin{proof}[of Lemma~\ref{lem2}]
According to the proof of Lemma 1 in \cite{lin2018consistency}, we have the following event
\begin{align*}
|\frac{1}{H}\sum_{h}\mu_h(\beta)^2  - \var\{{m}(\beta)\}| \leq \frac{1}{4\nu} \var\{{m}(\beta)\}
\end{align*} 
occurs with probability at least
\begin{align*}
1 - C_1 \exp[-C_2 \frac{n_0 \var\{{m}(\beta)\}}{H\nu^2} + C_3 \log{(H)}].
\end{align*}
Then with assumption \ref{ass1} we have
\begin{align*}
\sum_h \mu_h(\beta)^2 \geq C H s^{-\omega},
\end{align*}
Thus there exist a $h \in [H]$ such that 
\begin{align*}
|\mu_h(\beta)| \geq C_{\mu} s^{-\frac{\omega}{2}},
\end{align*}
thus the proof of Lemma \ref{lem2} is completed.
\end{proof}

The following lemma is from \cite{lin2018consistency}.

\begin{lemma}\label{lem4}
Let $x_1,..., x_n$ be $n$ i.i.d. samples from a p-dimensional sub-Gaussian random variable with covariance matrix $\Sigma$ and $\rho = p/n$. If there exists positive constants $C_1$ and $C_2$ such that
\begin{align*}
C_1 \leq \lambda_{\min}(\Sigma) \leq \lambda_{\max}(\Sigma) \leq C_2.
\end{align*}
Let $\widehat{\Sigma} = \frac{1}{n}\sum_i x_i x_i^{\T}$. Then
\begin{align*}
\|\widehat{\Sigma} - \Sigma\|_2 \rightarrow 0
\end{align*}
if $\rho = 0$ when $n \rightarrow \infty$.
It is also easy to see that, given the boundedness condition on $\Sigma$, we also have
\begin{align*}
\|\widehat{\Sigma} ^{-1} - \Sigma^{-1}\|_2 \rightarrow 0
\end{align*}
if $\rho \rightarrow 0$ when $n \rightarrow \infty$.
\end{lemma}

\begin{proof}[of Theorem~\ref{th:dp-vgm}]
According to (\ref{formular:dp}), it suffices to show
\begin{align}\label{error1}
\pr\{\widehat{m}_h(\mathcal{D}) + \xi \in \mathcal{O}\} \leq \pr\{\widehat{m}_h(\mathcal{D}^{\prime}) + \xi \in \mathcal{O}\} + \delta
\end{align}
for each pair of datasets $\mathcal{D}$, $\mathcal{D}^{\prime}$ differing in a single record and any possible output set $\mathcal{O}$, which is equivalent (see Lemma 3.17 in \citep{dwork2014algorithmic}) to 
\begin{align*}
\pr\left(\log{\left[\frac{\pr\{\widehat{m}_h(\mathcal{D}) + \xi \in \mathcal{O}\}}{\pr\{\widehat{m}_h(\mathcal{D}^{\prime}) + \xi \in \mathcal{O}\}}\right]} > \epsilon \right)  \leq \delta.
\end{align*}
Let $\psi = \widehat{m}_h(\mathcal{D}) - \widehat{m}_h(\mathcal{D}^{\prime})$, then the definition of $l_2$-sensitivity implies that $\|\psi \|_2 \leq \Delta_2 = {2R p^{1/2}}/{n}$. 
Notice
\begin{align*}
&\pr\left(\log{\left[\frac{\pr\{\xi \in \mathcal{O} - \widehat{m}_h(\mathcal{D})\}}{\pr\{\xi \in \mathcal{O} - \widehat{m}_h(\mathcal{D}^{\prime})\}}\right]} > \epsilon \right)  \leq \delta \\
\Longleftrightarrow
&\pr\left(\log{\left[\frac{\pr\{\xi \in \mathcal{O} - \widehat{m}_h(\mathcal{D})\}}{\pr\{\xi \in \mathcal{O} - \widehat{m}_h(\mathcal{D})  + \psi\}}\right]} > \epsilon \right)  \leq \delta \\
\Longleftrightarrow 
&\pr\left[\log{\left\{\frac{\int_{\mathcal{O} - \widehat{m}_h(X)} \exp{(-\frac{1}{2}\xi^{\T}\Sigma_{\xi}^{-1}\xi)}d\xi}{\int_{\mathcal{O} - \widehat{m}_h(X)} \exp{(-\frac{1}{2}(\xi+\psi)^{\T}\Sigma_{\xi}^{-1}(\xi+\psi))}d\xi}\right\}} > \epsilon \right] \leq \delta. \\
\end{align*}
If the above inequality holds for any point in set $\mathcal{O} - \widehat{m}_h(\mathcal{D})$, then it will hold for set $\mathcal{O} - \widehat{m}_h(\mathcal{D})$, thus we have
\begin{align*}
&\pr\left(\log{\left[\frac{\pr\{\xi \in \mathcal{O} - \widehat{m}_h(\mathcal{D})\}}{\pr\{\xi \in \mathcal{O} - \widehat{m}_h(\mathcal{D}^{\prime})\}}\right]} > \epsilon \right)  \leq \delta \\
\Longleftrightarrow 
&\pr\left\{|\frac{1}{2}\xi^{\T} \Sigma_{\xi}^{-1}\xi- \frac{1}{2}(\xi + \psi)^{\T} \Sigma_{\xi}^{-1}(\xi + \psi) > \epsilon \right\} \leq \delta \\
\Longleftrightarrow
&\pr\left(|\xi^{\T}\Sigma_{\xi}^{-1}\psi + \frac{1}{2}\psi^{\T}\Sigma_{\xi}^{-1}\psi| > \epsilon \right) \leq \delta.
\end{align*}
Let 
\begin{align*}
a = \xi^{\T}\Sigma_{\xi}^{-1}\psi+ \frac{1}{2}\psi^{\T}\Sigma_{\xi}^{-1}\psi,
\end{align*}
then we have $a \sim \mathcal{N}(\frac{1}{2}\psi^{\T}\Sigma_{\xi}^{-1}\psi, \psi^{\T}\Sigma_{\xi}^{-1}\psi)$. 
The behavior of Gaussian tails (\ref{tail1}) leads to
\begin{align}\label{error2}
\pr\left(|a - \frac{1}{2}\psi^{\T}\Sigma_{\xi}^{-1}\psi| > t \right) \leq 2\exp\left(-\frac{t^2}{2\psi^{\T}\Sigma_{\xi}^{-1}\psi}\right). 
\end{align}
Thus by setting $t = \epsilon - \frac{1}{2}\psi^{\T}\Sigma_{\xi}^{-1}\psi$, we need the following holds to guarantee the $(\epsilon, \delta)$-differential privacy,
\begin{align}\label{error3}
\nonumber 
&\delta \geq 2\exp(-\frac{t^2}{2\psi^{\T}\Sigma_{\xi}^{-1}\psi}) \\ \nonumber
\Longleftrightarrow 
&\log{\frac{2}{\delta}} \leq \frac{t^2}{2\psi^{\T}\Sigma_{\xi}^{-1}\psi} \\ \nonumber
\Longleftrightarrow 
&2 \psi^{\T} \Sigma_{\xi}^{-1}\psi\leq \frac{(\epsilon - \frac{1}{2}\psi^{\T}\Sigma_{\xi}^{-1}\psi)^2}{\log{\frac{2}{\delta}}} \\
\Longleftrightarrow 
&\frac{1}{4}(\psi^{\T}\Sigma_{\xi}^{-1}\psi)^2 - (2\log{\frac{2}{\delta}}+ \epsilon)\psi^{\T}\Sigma_{\xi}^{-1}\psi + \epsilon^2 \geq 0
\end{align}
By solving inequality (\ref{error3}), we have the following solution (the other solution is not reasonable since $\psi^{\T} \Sigma_{\xi}^{-1}\psi$ is bounded and small):
\begin{align*}
0 < \psi^{\T}\Sigma_{\xi}^{-1}\psi \leq 4\log{\frac{2}{\delta}} + 2\epsilon - 4\{(\log{\frac{2}{\delta}})^2 + \log{\frac{2}{\delta}}\epsilon\}^{1/2}.
\end{align*}
Thus we have
\begin{align*}
\|\Sigma_{\xi}^{-1}\|_2 &\leq \frac{4\log{\frac{2}{\delta}} + 2\epsilon - 4\{(\log{\frac{2}{\delta}})^2 + \log{\frac{2}{\delta}}\epsilon\}^{1/2}}{\Delta_2^2}.
\end{align*}
% As a result, 
% \begin{align*}
% 	\|V_{\xi}^{-1}\|_2 \leq \frac{4\log{\frac{2}{\delta}} + 2\epsilon - 4\{(\log{\frac{2}{\delta}})^2 + \log{\frac{2}{\delta}}\epsilon\}^{1/2}}{\Delta_{2}^2}.
% \end{align*}
Thus we complete the proof of Theorem \ref{th:dp-vgm}.
\end{proof}

\begin{proof}[of Theorem~\ref{ld-consistency1}]
Recall that
\begin{align*}
\widetilde{\Lambda} &= \widetilde{M}\widetilde{M}^{\T} = \left(\frac{\sum_{k=1}^{K}n_k \widehat{M}^{(k)}}{\sum_{k=1}^{K}n_k} + \frac{\sum_{k=1}^{K}n_k E_0^{(k)}}{\sum_{k=1}^{K}n_k}\right)\left(\frac{\sum_{k=1}^{K}n_k \widehat{M}^{(k)}}{\sum_{k=1}^{K}n_k} + \frac{\sum_{k=1}^{K}n_k E_0^{(k)}}{\sum_{k=1}^{K}n_k}\right)^{\T} \\
&\triangleq \left(\widehat{M} + E_0 \right) \left(\widehat{M} + E_0\right)^{\T} = \widehat{M} \widehat{M}^{\T} = \underbrace{\widehat{M} \widehat{M}^{\T}}_{I} + \underbrace{\widehat{M} E_0^{T}}_{II} + \underbrace{E_0 \widehat{M}^{\T}}_{III} +\underbrace{E_0 E_0^{\T}}_{IV},
%\widehat{{\Lambda}} &= \frac{1}{H}\left({M}_0 + {E}_0 \right)^{\T}\left({M}_0 + {E}_0 \right) \\
%&= \frac{1}{H} \sum_{h=1}^{H}\left({M}_{0h} + E_{0h}\right)^{\T}\left({M}_{0h} + E_{0h}\right) \\
%&= \frac{1}{H}\sum_{h=1}^{H}\left({M}_{0h}^{\T}{M}_{0h} + {M}_{0h}^{\T}E_{0h} + E_{0h}^{\T}{M}_{0h} + E_{0h}^{\T}E_{0h} \right) \\
%&= \underbrace{\frac{1}{H}\sum_{h=1}^{H}{M}_{0h}^{\T}{M}_{0h}}_{I} + \underbrace{\frac{1}{H}\sum_{h=1}^{H}{M}_{0h}^{\T}E_{0h}}_{II} + \underbrace{\frac{1}{H}\sum_{h=1}^{H}{M}_{0h}E_{0h}^{\T}}_{III} + \underbrace{\frac{1}{H}\sum_{h=1}^{H}E_{0h}^{\T} E_{0h}}_{IV}.
\end{align*}
where 
\begin{align*}
\widehat{M} = \frac{\sum_{k=1}^{K}n_k \widehat{M}^{(k)}}{\sum_{k=1}^{K}n_k} \quad\text{and}\quad E_0 = \frac{\sum_{k=1}^{K}n_k E_0^{(k)}}{\sum_{k=1}^{K}n_k}.
\end{align*}
Since we assume the sample sizes of all the slices are same, we have that $I = H^{-2} \sum_{h=1}^{H} \bar{x}_h \bar{x}_h^{\T}$. For $I$, by the result of Theorem 2 in \cite{lin2018consistency}, we have
\begin{align*}
\|\widetilde{M}\widetilde{M}^{\T}  - \Lambda_p\|_2 = O_p\left(\frac{1}{H^{\nu+1}} + \frac{H p}{N} + {\frac{p^{1/2}}{N^{1/2}}}\right)
\end{align*}
as long as $N$ is sufficient large.

For $IV$, first $E_0$ follow the Gaussian distribution, we assume $E_0 \sim \mathcal{N}(0, \Sigma_0)$, then it can be implied that 
\begin{align*}
\mathbb{E}\left( \frac{1}{H}\sum_{h=1}^{H}E_{0h} E_{0h}^{\T}\right) = \Sigma_0,
\end{align*}
where $E_{0h}$ is the $h$th column of $E_0$. By Lemma \ref{lemA2}, we have 
\begin{align*}
\|\frac{1}{H}\sum_{h=1}^{H} E_{0h}E_{0h}^{\T} - \Sigma_0\|_2 \leq C \tau_1^2 \left\{\left({\frac{p+\mu}{H}}\right)^{1/2} + \frac{p + \mu}{H}\right\}\|\Sigma_0\|_2,
\end{align*}
holds with probability $1 - 2e^{-\mu}$, where $\tau_1 \geq 1$ is a constant such that
\begin{align*}
\|\left \langle E_{0h},x \right \rangle \|_{\psi} \leq \tau_1 \|\left \langle E_{0h},x \right \rangle\|_{L^2}.
\end{align*}
Thus
\begin{align}\label{thm31}
\|E_0 E_0^{\T} - H \Sigma_0\|_2 \leq C \tau_1^2 \left\{\left({\frac{p+\mu}{H}}\right)^{1/2} + \frac{p + \mu}{H}\right\}\|H \Sigma_0\|_2.
\end{align}
By the result of Theorem \ref{th:dp-vgm}, we have
\begin{align*}
\|\Sigma_0\|_2 &= \|\frac{\sum_{k=1}^{K}n_k U_k^{\T}S_kU_k}{H^2 \sum_{k=1}^{K}n_k}\|_2 \\
%&\leq \frac{1}{K^2} \sum_{k=1}^{K} \|U_k S_k U_k \|_2 \leq \frac{1}{K^2} \sum_{k=1}^{K}\|S_k\|_2\\
&\leq  \max_{k} \frac{n_k}{H^2 N}\|S_k\|_2 \leq \frac{C R^2 p \log{\frac{2}{\delta}}}{H^2 n_{\epsilon, \delta, p, R}^2 \epsilon^2},
\end{align*}
where the last inequality follows from the result of Theorem \ref{th:dp-vgm}. Combining (\ref{thm31}), we have
\begin{align*}
\|E_0 E_0^{\T} - H \Sigma_0\|_2 \leq \frac{C \tau_1 ^2 R^2 p \log{\frac{2}{\delta}}}{H n_{\epsilon, \delta, p, R}^2 \epsilon^2} \left\{\left({\frac{p+\mu}{H}}\right)^{1/2} + \frac{p + \mu}{H}\right\},
\end{align*}
it can be implied that
\begin{align*}
\|E_0 E_0^{\T}\|_2 &\leq \frac{C \tau_1 ^2 R^2 p \log{\frac{2}{\delta}}}{H n_{\epsilon, \delta, p, R}^2 \epsilon^2} \left\{\left({\frac{p+\mu}{H}}\right)^{1/2} + \frac{p + \mu}{H}\right\} + \frac{C \tau_1 ^2 R^2 p \log{\frac{2}{\delta}}}{H n_{\epsilon, \delta, p, R}^2 \epsilon^2}.
\end{align*}
since we choose a larger $\mu$ such that 
\begin{align*}
\tau_1^2\left\{\left({\frac{p+\mu}{H}}\right)^{1/2} + \frac{p + \mu}{H}\right\} \gg 1,
\end{align*}
and
\begin{align*}
\frac{C \tau_1 ^2 R^2 p \log{\frac{2}{\delta}}}{H n_{\epsilon, \delta, p, R}^2 \epsilon^2} \left\{\left({\frac{p+\mu}{H}}\right)^{1/2} + \frac{p + \mu}{H}\right\} = o(\frac{1}{H^{\nu + 1}}).
\end{align*}
Then we have 
\begin{align*}
\|E_0 E_0^{\T}\|_2 = o_p(\frac{1}{H^{\nu+1}}).
\end{align*}

For $II$ and $III$, Let
\begin{align*}
D = \widehat{M}E_0^{\T},
\end{align*}
and we will show the properties of $D_{ij}$. Since the rows of $\widehat{M}$ and $E_{0}$ are independent. By (\ref{hoeffding}), we have
\begin{align}\label{thm32}
\pr\left( |D_{ij}| \geq t\right) \leq 2\exp\left( - \frac{c H t^2}{\tau_2^2 R^2}\right),
\end{align}
where $\tau_2 = \max_i(\|{E}_{0h,i}\|_{\psi})$. We will first present the magnitude of $\tau_2$. Since $E_{0h}$ is Gaussian, then all $E_{0h,i}$ obey the Gaussian distribution too and the variance is $\Sigma_{0,ii}$. By the result in Theorem \ref{th:dp-vgm}, we have
\begin{align*}
\tau_2^2 = \max_i(\|{E}_{0h,i}\|_{\psi})^2  \leq C \|\Sigma_0\|_2
\leq \frac{C R^2 p \log{\frac{2}{\delta}}}{H^2 n_{\epsilon, \delta, p, R}^2 \epsilon^2}.
\end{align*}
By choosing $t = \{H^{(\nu+1)}p\}^{-1}$ we have
\begin{align*}
\pr\left\{ |D_{ij}| \geq \frac{1}{H^{(\nu+1)}p}\right\} \leq 2\exp\left( - \frac{c n_{\epsilon,\delta,p,R}^2 \epsilon^2}{R^4 H^{2\nu -1}p^3 \log{\frac{2}{\delta}}}\right) \rightarrow 0
\end{align*}
by assumption. In conclusion, it can be implied that
\begin{align*}
\|D\|_2 \leq \|D\|_F \leq \frac{1}{H^{\nu+1}}
\end{align*}
with probability tending to 0.

Thus we completed the proof of Theorem \ref{ld-consistency1}.
\end{proof}

\begin{proof}[of Lemma~\ref{lem3}]
First, we will show the bound for $\|\widetilde{\Sigma} - \frac{1}{n}X X^{\T}\|_2$. According to (\ref{tail1}), we have
\begin{align*}
\pr\{|A_{ij}| > t\} \leq \exp\left(- \frac{ct^2}{\omega^2}\right).
\end{align*}
Since
\begin{align*}
\frac{1}{N{\epsilon}^{1/2}} \ll \frac{p+1}{N \epsilon}\left\{2\log{\left(\frac{p^2 +p}{2\delta\sqrt{2\pi}} \right)}\right\}^{1/2},
\end{align*}
it can be implied that 
\begin{align*}
\pr(|A_{ij}| > t) \leq \exp\left\{- \frac{cn^2\epsilon^2t^2}{p^2 \log{\left(\frac{p^2 +p}{2\delta\sqrt{2\pi}} \right)}}\right\}.
\end{align*}
Then we have
\begin{align*}
\|A\|_2 \leq \|A\|_F \leq \frac{p^2}{n^\alpha}
\end{align*}
holds with probability at least $1 - p^2\exp\left\{- \frac{cN^{(2 - 2\alpha)}\epsilon^2}{p^2 \log{\left(\frac{p^2 +p}{2\delta\sqrt{2\pi}} \right)}}\right\}$, where $0 < \alpha < 1$. Since $\|\sum_{k=1}^{K}(c_R^{(k)})^2 A \|_2\leq \|K \max_k (c_R^{(k)})^2 A\|_2 \rightarrow 0$ in the low-dimensional settings. Thus we have
\begin{align*}
\|\widetilde{\Sigma} - \Sigma\|_2 \leq \|\Sigma - \frac{1}{N} X X^{\T}\|_2 + \|\sum_{k=1}^{K}(c_R^{(k)})^2 A\|_2 \rightarrow 0
\end{align*}
as $N \rightarrow \infty$ by Lemma \ref{lem4}. According to Lemma \ref{lemA3}, we have
\begin{align*}
\lambda_{\min}\left(\frac{1}{N}X X^{\T}\right) + \lambda_{\max}(\sum_{k=1}^{K}(c_R^{(k)})^2 A)\geq \lambda_{\min}(\widetilde{\Sigma}) \geq \lambda_{\min}\left(\frac{1}{N}X X^{\T}\right) + \lambda_{\min}(\sum_{k=1}^{K}(c_R^{(k)})^2 A),
\end{align*}
then
\begin{align*}
\|\widetilde{\Sigma}^{-1} - \left(\frac{1}{N}X X^{\T}\right)^{-1}\|_2 \leq \|\sum_{k=1}^{K}(c_R^{(k)})^2 A\|_2 \rightarrow 0,
\end{align*}
thus we have
\begin{align*}
&\|\widetilde{\Sigma}^{-1} - \Sigma^{-1}\|_2 \\
=&\|\widetilde{\Sigma}^{-1} - \left(\frac{1}{N}X X^{\T}\right)^{-1} + \left(\frac{1}{N}X X^{\T}\right)^{-1} - \Sigma^{-1}\|_2 \\
\leq& \|\widetilde{\Sigma}^{-1} - \left(\frac{1}{N}X X^{\T}\right)^{-1}\|_2 + \|\left(\frac{1}{N}X X^{\T}\right)^{-1} - \Sigma^{-1}\|_2,
\end{align*}
where the last term is proved to coverage to 0 when $N \rightarrow \infty$ in Lemma \ref{lem4}. Thus we complete the proof of Lemma \ref{lem3}.
\end{proof}

\begin{proof}[of Theorem~\ref{ld-consistency2}]
\begin{align*}
&\|\widehat{\Sigma}^{-1}\widehat{\Lambda} - \Sigma^{-1}\Lambda_p\|_2 \\
\leq &\|\widehat{\Sigma}^{-1} - \Sigma^{-1}\|_2 \|\widehat{\Lambda}^{-1}\|_2 + \|\Sigma\|_2 \|\widehat{\Lambda} - \Lambda_{p}\|_2,
\end{align*}
which $\rightarrow 0$ when $\frac{p}{N} \rightarrow 0$ as $N \rightarrow \infty$ by Lemma \ref{lem3}. Thus we complete the proof of Theorem \ref{ld-consistency2}.
\end{proof}

\begin{proof}[of Proposition~\ref{prop:scr}]

Recall that
\begin{align*}
\mathcal{T} = \left\{j| {E}\{x(j)|y\} \quad\text{is not a constant} \right\},
\end{align*}
\begin{align*}
\mathcal{I}_h = \left\{ j| |\bar{x}_h (j)| > t \right\}, h = 1,..., H.
\end{align*}
\begin{align*}
\mathcal{I} = \cup_h \mathcal{I}_h = \left\{ j|\text{there exists a} \quad h \in [1,H], \text{s.t.}\quad |\bar{x}_h (j)| > t\right\},
\end{align*}
\begin{align*}
\mathcal{I}^{c} = \left\{j|\text{for all}\quad h \in [1, H], \quad |\bar{x}_h(j)| < t \right\},
\end{align*}
and $|\mathcal{T}| \leq cs$. Since ${E}\{x(j)|y\} = 0$, we have ${E}\{x(j)|_{y \in S_h}\} = 0$. Together with Lemma \ref{lem1} and \ref{lem2} we have
\begin{align*}
\pr(\mathcal{T} \subset \mathcal{I}) &\geq \pr[\cap_{j \in \mathcal{T}}\left\{\text{there exists a} \quad h \in [1,H], \text{s.t.}\quad |\bar{x}_h (j)| > t\right\}] \\
&\geq 1 - \sum_{j \in \mathcal{T}}\pr\left\{\text{for all}\quad h \in [1, H], \quad |\bar{x}_h(j)| < t\right\} \\
&\geq \left[1 - \sum_{j \in \mathcal{T}}\pr\left\{\text{for all}\quad h \in [1, H], \quad |\mu_h(j)| < C_{\mu}s^{-\frac{\omega}{2}}\right\}\right]\\
&\left[ \sum_{j \in \mathcal{T}}\pr\left\{\text{for all}\quad h \in [1, H], \quad |\bar{x}_h(j) - \mu_h(j)|< C s^{-\frac{\omega}{2}}\right\}\right] \\
&\geq 1 -  C_1 \exp\left\{-C_2 \frac{n_{\epsilon,\delta,s,R} s^{-\omega}}{H\nu^2} + C_3 \log{(H)}+ C_4 \log{(s)}\right\}\\
&- C_5 \exp \left\{\frac{-n_{\epsilon,\delta,s,R} s^{-\omega}}{2 C H \tau ^{2}+2 s^{-\frac{\omega}{2}} \tau} + C_6 \log{(s)} + C_7 \log{(H)}\right\}.
\end{align*}
And 
\begin{align*}
\pr(\mathcal{T}^c \subset \mathcal{I}^c) &\geq 1 - \sum_{j \in \mathcal{T}^c}\pr\left\{\text{for all} \quad h \in [1,H], |\bar{x}_h(j)| >t \right\} \\
&\geq \left[1 - \sum_{j \in \mathcal{T}^c}\pr\left\{\text{for all} \quad h \in [1,H], |\mu_h(j)| > C_{\mu}s^{-\frac{\omega}{2}} \right\}\right] \\
&\left[\sum_{j \in \mathcal{T}^c}\pr\left\{\text{for all} \quad h \in [1,H], |\bar{x}_h(j) - \mu_h(j)| < C_{\mu}s^{-\frac{\omega}{2}} \right\}\right] \\
&\geq 1 - C_1 \exp \left\{\frac{-n_{\epsilon,\delta,s,R} s^{-\omega}}{2 C H \tau ^{2}+2 s^{-\frac{\omega}{2}} \tau} + C_2 \log{(H)} + C_3 \log{(p - cs)}\right\}.
\end{align*}
The last inequality is because ${E}\{x(j)|_{y \in S_h}\} = 0$, as a result
\begin{align*}
\pr\left\{\text{for all} \quad h \in [1,H], |\mu_h(j)| > C_{\mu}s^{-\frac{\omega}{2}} \right\} = 0.
\end{align*}
Thus we complete the proof of Proposition \ref{prop:scr}.
\end{proof}

\begin{proof}[of Theorem~\ref{thm:scr}]
Let $p_1 = \pr(j \notin \mathcal{I}|j \in \mathcal{T})$, then by the proof of Proposition \ref{prop:scr}, we have
\begin{align*}
p_1 \leq  C_1 \exp\left\{-C_2 \frac{n_{\epsilon,\delta,s,R} s^{-\omega}}{H\nu^2} + C_3 \log{(H)}\right\}
+ C_4 \exp \left\{\frac{-n_{\epsilon,\delta,s,R} s^{-\omega}}{2 C H \tau ^{2}+2 s^{-\frac{\omega}{2}} \tau} + C_5 \log{(H)}\right\}.
\end{align*}
Let $p_2 = \pr(j \in \mathcal{I}|j \notin \mathcal{T})$, similarly we have
\begin{align*}
p_2 \leq  C_1 \exp \left\{\frac{-n_{\epsilon,\delta,s,R} s^{-\omega}}{2 C H \tau ^{2}+2 s^{-\frac{\omega}{2}} \tau} + C_2 \log{(H)}\right\}.
\end{align*}
Then
\begin{align*}
&\pr\{j \in \mathcal{T}, \text{frequency less than} \quad {K/2}\}\\
=& \mathrm{C}_{K}^{K/2}p_1^{K/2}(1 - p_1)^{K/2}+...+ \mathrm{C}_{K}^K p_1^{K}(1 - p_1)^0 \\
\leq& \frac{K}{2}\mathrm{C}_{K}^{K/2}p_1^{K/2}(1 - p_1)^{K/2} \\
\leq &C \frac{K}{2}\sqrt{2\pi K}(\frac{K}{e})^{K} p_1^{K/2} \leq C K^{3/2} (\frac{K^2 p_1}{e^2})^{K/2}.
\end{align*}
where the second inequality follows from Stirling's approximation. Then we have
\begin{align*}
\pr(\mathcal{T} \subset \mathcal{T}_0) \geq 1 - C s K^{3/2} (\frac{K^2 p_1}{e^2})^{K/2}.
\end{align*}
Similarly, 
\begin{align*}
&\pr\{k \notin \mathcal{T}, \text{frequency more than} \quad {K/2}\} \\
=&\mathrm{C}_{K}^{K/2}p_2^{K/2}(1 - p_2)^{K/2}+...+ \mathrm{C}_{K}^K p_2^{K}(1 - p_2)^0 \\
\leq&C K^{3/2} (\frac{K^2 p_2}{e^2})^{K/2}.
\end{align*}
Thus we have
\begin{align*}
\pr(\mathcal{T}^c \subset \mathcal{T}_0^{c}) \geq 1 - C p K^{3/2} (\frac{K^2 p_2}{e^2})^{K/2}.
\end{align*}
Thus we complete the proof of Theorem \ref{thm:scr}.
\end{proof}

\begin{proof}[of Theorem~\ref{hd-consistency1}]
From Theorem \ref{thm:scr}, we have 
\begin{align*}
P(\mathcal{T}_0 = \mathcal{T}) \rightarrow 1.
\end{align*}
When $\mathcal{T}_0 = \mathcal{T}$, we have $\mathcal{T}_0 = O(s)$, then we have
\begin{align*}
\|e(\widehat{\Lambda}^{\mathcal{T}_0 , \mathcal{T}_0}) - \Lambda\|_2 \leq \|\widehat{\Lambda}^{\mathcal{T}_0 , \mathcal{T}_0} - \Lambda^{\mathcal{T}_0, \mathcal{T}_0}\|_2 = O_p\left(\frac{1}{H^{\nu+1}} + \frac{H s}{N} + {\frac{ s^{1/2}}{N^{1/2}}}\right)
\end{align*}
according to the results in Theorem \ref{ld-consistency1}. In particular, with probability converging to 1 we have 
\begin{align*}
\|e(\widehat{\Lambda}^{\mathcal{T}_0 , \mathcal{T}_0}) - \Lambda\|_2 \rightarrow 0.
\end{align*}
Thus we complete the proof of Theorem \ref{hd-consistency1}.

\end{proof}

\begin{lemma}\label{lem5}
Under condition \ref{con1} - \ref{con6} and assumption \ref{ass1}, we have
\begin{align*}
\|\widehat{\Sigma}^{\mathcal{T}_0, \mathcal{T}_0} - \Sigma^{\mathcal{T}_0, \mathcal{T}_0}\|_2 \rightarrow 0
\end{align*}
when $n \rightarrow \infty$. It is also easy to see that
\begin{align*}
\|(\widehat{\Sigma}^{\mathcal{T}_0, \mathcal{T}_0})^{-1} - (\Sigma^{\mathcal{T}_0, \mathcal{T}_0})^{-1}\|_2 \rightarrow 0.
\end{align*}
\end{lemma}

\begin{proof}[of Lemma~\ref{lem5}]
The proof is almost identical to the proof of Lemma \ref{lem3}, we only need to replace the dimension $p$ with sparsity $s$.
\end{proof}

\begin{proof}[of Theorem~\ref{hd-consistency2}]
Since
\begin{align*}
&\|e\left\{(\widehat{\Sigma}^{\mathcal{T}_0, \mathcal{T}_0})^{-1}\widehat{\Lambda}^{\mathcal{T}_0 , \mathcal{T}_0}\right\} - e\left\{(\Sigma^{\mathcal{T}_0, \mathcal{T}_0})^{-1}\Lambda^{\mathcal{T}_0, \mathcal{T}_0}\right\}\|_2 \\
\leq &\|(\widehat{\Sigma}^{\mathcal{T}_0, \mathcal{T}_0})^{-1}\widehat{\Lambda}^{\mathcal{T}_0 , \mathcal{T}_0} - (\Sigma^{\mathcal{T}_0, \mathcal{T}_0})^{-1}\Lambda^{\mathcal{T}_0, \mathcal{T}_0}\|_2.
\end{align*}
According to the same procedures in the proof of Theorem \ref{ld-consistency2}, we can get the conclusions of Theorem \ref{hd-consistency2}.
\end{proof}

We have assumed that the errors $\omega$ are independent and identically distributed sub-Gaussian random variables with parameter $\tau^2$. In this appendix we summarize some properties of sub-Gaussian random variables.

A sub-Gaussian random variable $Z$ satisfies the following tail probability bounds:
\begin{align}\label{tail1}
P(|Z|>t)\leq 2\exp(-t^2/2\tau^2)\text{for all }t>0
\end{align}
We refer to the sub-Gaussian parameter of $Z$ as the smallest $\tau^2$ satisfying (\ref{tail1}). Following [\citet{Vershynin12},Lemma 5.5] we observe that there exists universal constants $m$ and $M$ such that $m\|Z\|_{\psi}\leq \tau^2 \leq M\|Z\|_{\psi}^2$. We note that if $\omega=(\omega_1,\omega_2,...\omega_n)^{\prime}$ that $\omega_i$'s are independent zero-centered sub-Gaussian random variables, then weighted sums of $\omega_i$ are also sub-Gaussian and satisfy an useful property [\citet{Vershynin12},Lemma 5.5]:
\begin{align}\label{tail2}
\|v^{\prime}\omega\|_{\psi}^2 \leq K\|v\|_2^{2}\max_{i}(\|\omega_{i}\|_{\psi}^2)
\end{align}
where $K$ is an absolute constant. And we have the following General Hoeffding's inequality [\citet{Vershynin18}, Theorem 2.6.3]
\begin{align}\label{hoeffding}
P\left(|v^{\prime}\omega| \geq t\right) \leq 2 \exp\left(- \frac{ct^2}{\max_{i}(\|\omega_{i}\|_{\psi}^2)\|v\|_2^2}\right)
\end{align}

We now state some useful results for random matrices, the following lemma is Theorem 4.6.1 in \cite{Vershynin18}:

\begin{lemma}\label{lemA1}
Let $A$ be an $m \times n$ matrix whose rows $A_i$ are independent, mean zero, sub-gaussian isotropic random vectors in $\mathbb{R}^n$. Then for any $t \geq 0$ we have
\begin{align*}
\|\frac{1}{m}A^{\T}A - I_{n}\|_2 \leq \left(\max_i \|A_i\|_{\psi}\right)^2 \max(\delta, \delta^2)
\end{align*}
holds with probability at least $1 -  2 \exp(-t^2)$, where $\delta = C\left({n^{1/2}/{m^{1/2}}} + {t}/{{m}^{1/2}}\right)$.
\end{lemma}

We need an another lemma which is a corollary of Lemma \ref{lemA1}.

\begin{lemma}\label{lemA2}
Let $Z$ be a sub-gaussian random vector in $\mathbb{R}^n$, $\Sigma = {E} Z Z^{\T}$ and $\Sigma_m = \frac{1}{m} \sum_{i=1}^{m} Z_i Z_i^{T}$. More precisely, assume that there exists $B \geq 1$ such that 
\begin{align}\label{A21}
\|\left \langle Z, z\right \rangle\|_{\psi} \leq B \|\left \langle Z, z\right \rangle\|_{L^2}
\end{align}
for any $z \in \mathbb{R}^n$. Then for every positive integer $m$, we have
\begin{align*}
\|\Sigma_m - \Sigma\|_2 \leq C B^2 \left\{ \left(\frac{n + \mu}{m}\right)^{1/2} + \frac{n+\mu}{m}\right\}\|\Sigma\|_2
\end{align*}
holds with probability at least $1 -2e^{-\mu}$.
\end{lemma}

\begin{proof}[of Lemma~\ref{lemA2}]

Let us bring the random vectors $Z$, $Z_1,..., Z_m$ to the isotropic position. There exist isotropic random vectors $V, V_1, ... V_m$ such that 
\begin{align*}
Z = \Sigma^{1/2} V \quad \text{and} \quad  Z_i = \Sigma^{1/2} V_i.
\end{align*}
The sub-Gaussian assumption (\ref{A21}) then implies that
\begin{align*}
\|V\|_{\psi} \leq B \quad \text{and} \quad \|V_i\|_{\psi} \leq B.
\end{align*}
Then
\begin{align*}
\|\Sigma_m - \Sigma\|_2 = \|\Sigma^{1/2} R_m \Sigma^{1/2}\|_2 \leq \|R_m\|_2 \|\Sigma\|_2,
\end{align*}
where $R_m = \frac{1}{m}\sum_{i=1}^{m}V_iV_i^{\T} - I_n$. What's more, we have
\begin{align*}
{n}^{1/2} + {\mu}^{1/2} \leq {2^{1/2}(n + \mu)^{1/2}},
\end{align*}
and
\begin{align*}
({n}^{1/2} + {\mu}^{1/2})^2 \leq 2 (n + \mu).
\end{align*}
Combining the above results with Lemma \ref{lemA1}, we can proof Lemma \ref{lemA2}.
\end{proof}

Weyl 's inequality (\cite{Weyl12}):

\begin{lemma}\label{lemA3}
Let ${M} = N + R$, and $R$ be $n \times n$ Hermitian matrices, with their respective eigenvalues $\mu_i, \nu_i, \rho_i$ ordered as follows:
\begin{align*}
{M}: & \mu_{1} \geq \cdots \geq \mu_{n} \\
N: & \nu_{1} \geq \cdots \geq \nu_{n} \\
R: & \rho_{1} \geq \cdots \geq \rho_{n} .
\end{align*}

Then the following inequalities hold:
\begin{align*}
\nu_i + \rho_n \leq \mu_i \leq \nu_i + \rho_1, \quad i = 1,...,n.
\end{align*}
\end{lemma}
